# Supplementary material for: Simulation of left ventricle fluid dynamics with mitral regurgitation from magnetic resonance images with fictitious elastic structure regularization
Source: arXiv:1707.03998 source file (2017-07-13)
Supplement: Supplementary file 1 [file appendix.tex]

\rev{In this section we compare the results obtained with a fluid-structure interaction simulation using a fictitious elastic structure to impose the ventricle motion against
imposing directly the motion of the fluid domain using Navier-Stokes equations in an ALE formulation.}
